# Supplementary material for: Behavioral QLTL
Source: arXiv:2102.11184 source file (2021-02-22)
Supplement: Supplementary file 1 [file appendix.tex]

\section{Appendix}
